# Supplementary material for: LEMIX: Enabling Testing of Embedded Applications as Linux Applications (Extended Report)
Source: arXiv:2503.17588 source file (2025-06-12)
Supplement: Supplementary file 1 [file evaluation_additional_instrumentation.tex]

\begin{figure}[t]
\centering
 \includegraphics[scale=0.5]{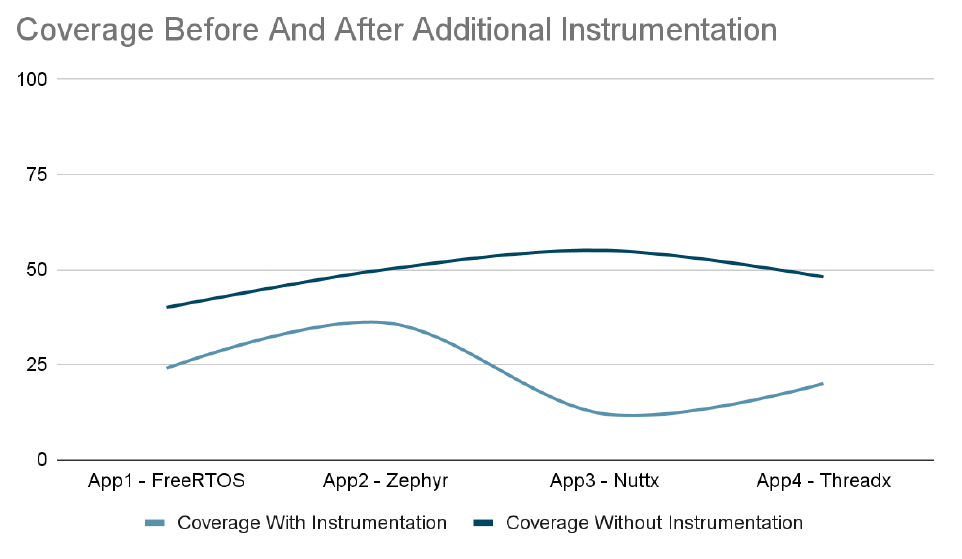}
\caption{Placeholder line chart representing the improvements in coverage with additional instrumentation.}
\label{fig:eval_additional_ins}
\end{figure}
